# Supplementary material for: FairTraDEX: A Decentralised Exchange Preventing Value Extraction
Source: arXiv:2202.06384 source file (2022-08-04)
Supplement: Supplementary file 1 [file ProtocolFlow.tex]

\newpage

\section{Protocol Flow}\label{app:ProtocolFlow}

Client Protocol Flow: \\

\begin{center}
\scalebox{0.5}{
$\begin{array}{c c c}
    \text{\textsf{Client}} \ \client & & \protocolContract \\
    \hline
    \hline
    & \textbf{Register} & \\
    \commSerialNum, \commRandomness \gets \text{genZKInfo}() & &  \\
    \regToken \assign \commit(\commSerialNum, \commRandomness) & &  \\
    & \underset{\bitcoin: \ \escrowClient+ \feeRelayer}{\xrightarrow{\hspace{1em}  \ \regToken \hspace{1em}}} &  \\
    & & \clients\getAppend(\regToken) \\
    \hline
     & \textbf{Commit} & \\
    \token \in \{\tokenA, \tokenB\}& & \\
    \tokenAmount \in \mathbb{R}_{>0}& & \\
    \tokenPrice \in \mathbb{R}_{>0} \cup \{\marketOrder\}& & \\
    \width \in \mathbb{R}_{\geq 1}& & \\
    \commitment \gets \commit(\token, \tokenAmount, \tokenPrice, \width) & &\\
    \proofZK \gets \text{genZKProof}(\regToken, \clients,*) & &  \\
    & \xrightarrow{\hspace{1em} \relay(\tagClientCommit, \commitment, \commSerialNum, \proofZK) \hspace{1em}}& \\
    &  & \clientCommits\getAppend([\commSerialNum,\commitment]) \\
    \hline
     & \textbf{Reveal} &  \\
    \text{leave} \in \{0,1\}& &   \\
    \commSerialNum', \commRandomness' \gets
    \begin{cases}
    \begin{array}{l l}
    \varnothing, & \text{if}\ \text{leave}=1 \\
    \text{genZKInfo}(), & \text{if}\ \text{leave}=0
    \end{array}
    \end{cases} 
    & & \\
    \regTokenNew \gets
    \begin{cases}
    \begin{array}{l l}
    \varnothing, & \text{if}\ \text{leave}=1 \\
    \commit(\commSerialNum', \commRandomness'), & \text{if}\ \text{leave}=0
    \end{array}
    \end{cases} 
    & & \\
    & \underset{\begin{array}{l l}
    \tokenA: \ \textit{minimum}(\tokenAmount, \tokenAMaxSizeClient), & \text{if}\ \token =\tokenA \\
    \tokenB: \ \textit{minimum}(\tokenAmount, \tokenBMaxSizeClient), & \text{if}\ \token =\tokenB \\
    \bitcoin: \ \feeRelayer, & \text{if} \ \regTokenNew = \varnothing
    \end{array}}{\xrightarrow{\hspace{1em}
     : \ \tagClientReveal,\token, \tokenAmount, \width, \tokenPrice, \ \commSerialNum, \commRandomness, \regToken, \regTokenNew 
    \hspace{1em}}}  & \\
    & & \revealedOrders\getAppend([\client, \token, \tokenAmount,  \tokenPrice, \width])  \\
    &  & \clients\remove(\regToken) \\
    & & \clientCommits\remove(\commSerialNum)\\
    & & \clients\getAppend(\regTokenNew), \ \text{if}\ \regTokenNew \neq \varnothing \\
    & \underset{\bitcoin: \ \feeRelayer \ \text{if} \ \regTokenNew=\varnothing}{\xrightarrow{\hspace{6em}}} & \\
    & \underset{\bitcoin: \ \escrowClient \ \text{if} \ \regTokenNew=\varnothing}{\xleftarrow{\hspace{6em}}} & \\
    \hline
     & \textbf{Resolution} & \\
    & & \clearingPrice \assign \textit{getClearingPrice}(\revealedOrders) \\
    & & \tokenTradeSize \assign \textit{getClearingVolume}(\clearingPrice, [\token, \tokenAmount,  \tokenPrice, \width], \revealedOrders)\\
    &  \underset{\begin{array}{l l}
    \tokenB: \ \tokenTradeSize, & \text{if}\ \token =\tokenA, \\
    \tokenA: \ \tokenTradeSize, & \text{if}\ \token =\tokenB .
    \end{array}}{\xleftarrow{\hspace{6em} }} & \\
    & & \textit{leftovers} \assign \begin{cases}
    \begin{array}{l l}
    \tokenAmount- \frac{\tokenTradeSize}{\clearingPrice}, & \text{if}\ \token = \tokenA \\
    \tokenAmount- (\tokenTradeSize \cdot \clearingPrice), & \text{if}\ \token = \tokenB
    \end{array}
    \end{cases}  \\
    & \underset{\begin{array}{l l}
    \tokenA: \ \textit{leftovers}, & \text{if}\ \token =\tokenA, \\
    \tokenB: \ \textit{leftovers}, & \text{if}\ \token =\tokenB.
    \end{array}}{\xleftarrow{\hspace{6em} }} & \\
    \hline
    \end{array}$}    
\end{center}

MM Protocol Flow: \\
\\

\scalebox{0.55}{
$\begin{array}{c c c}
    \protocolContract & & \text{\textsf{Market Maker}} \ \MM \\
    \hline
    \hline
    & \textbf{Commit} & \\
    & & \MMBidPrice  \in \mathbb{R}_{>0} \\
    & &  \MMBidAmount \in \mathbb{R}_{>0} \\
    & & \MMOfferPrice  \in \mathbb{R}_{>0} \\
    & & \MMOfferAmount  \in \mathbb{R}_{>0} \\
    & & \commitment \gets \commit(\MMBidPrice, \ \MMBidAmount, \ \MMOfferPrice,  \ \MMOfferAmount)  \\
    & \underset{\bitcoin: \ \escrowMM}{\xleftarrow{\hspace{1em} \
    \tagMMCommit, \commitment 
    \hspace{1em}}} & \\
    \MMCommits\getAppend([\MM, \commitment])& & \\
    \hline \\
    & \textbf{Reveal} &  \\
    & &  \\
    & \underset{\bitcoin: \ \escrowMM}{\xrightarrow{\hspace{6em}}}  & \\
    & & x \assign  \textit{minimum}(\MMBidAmount, \tokenAMaxSizeClient)   \\
    & & y \assign  \textit{minimum}(\MMOfferAmount, \tokenBMaxSizeClient) \\
    & \underset{\tokenA: \ x, \ \tokenB: \ y }{\xleftarrow{\hspace{1em}  \ \tagMMReveal,\MMBidPrice, \ \MMBidAmount, \ \MMOfferPrice,  \ \MMOfferAmount \hspace{1em}}}  & \\
    \tightestWidth \assign \frac{\MMOfferPrice}{\MMBidPrice}, \ \text{if} \ \big( \frac{\MMOfferPrice}{\MMBidPrice}<\tightestWidth \ \logicalOr \ \tightestWidth = \any \big) & & \\
    \revealedOrders\getAppend([ \MM, \tokenA, x,  \MMBidPrice, \any ]) & & \\
    \revealedOrders\getAppend([ \MM, \tokenB,  y,  \MMOfferPrice, \any ]) & & \\
    \MMCommits\remove(\MM) & & \\
    \hline
     & \textbf{Resolution} & \\
     \clearingPrice \assign \textit{getClearingPrice}(\revealedOrders) & & \\
    \tokenTradeSize_B \assign \textit{getClearingVolume}(\clearingPrice, [ \tokenA,  x,  \MMBidPrice, \any], \revealedOrders) & & \\
    \textit{bidLeftovers} \assign x - \frac{\tokenTradeSize_A}{\clearingPrice} & &  \\
    \tokenTradeSize_A \assign \textit{getClearingVolume}(\clearingPrice, [ \tokenB,  y,  \MMOfferPrice, \any], \revealedOrders) & & \\
    \textit{offerLeftovers} \assign y - (\tokenTradeSize_A \cdot \clearingPrice) & &  \\
    & \underset{\begin{array}{l l}
    \tokenA: \ \tokenTradeSize_A + \ \textit{bidLeftovers} \\
    \tokenB: \ \tokenTradeSize_B + \ \textit{offerLeftovers}.
    \end{array}}{\xrightarrow{\hspace{6em} }} & \\
    & & \\
    \hline
    \end{array}$}
